# Supplementary material for: Unsupervised Coordinate-Based Video Denoising
Source: arXiv:2307.00179 source file (2023-07-01)
Supplement: Supplementary file 1 [file supplement.tex]

% \vspace{130mm}
\section{Network Architecture and Training}
\begin{table}[h]
    % \small
    \begin{center}
    \begin{tabular}{ccc}
     \hline
     \centering
      Name &  $N_{out}$  & Function\\ 
      \hline
      Input &  $2(x*L)+x$  & $\gamma(p_t)$  \\ 
      conv\_0 &  256  & Convolution 1 x 1 \\
      conv\_1 &  256  & Convolution 3 x 3 \\
      conv\_2 &  256  & Convolution 3 x 3 \\
      conv\_3 &  256  & Convolution 3 x 3 \\
      conv\_4 &  256  & Convolution 3 x 3 \\
      conv\_5 &  C  & Convolution 3 x 3 \\
     \hline
    \end{tabular}
    \end{center}
\caption{\textbf{Network architecture of the feature generator}}
\label{tab:feat}
\end{table}
As described in Table \ref{tab:feat}, the feature generator $\mathcal{F}_\theta$ takes as input a batch of sampled coordinated grids $\{G_t | t = 1,...,B\}$ of the corresponding batch of noisy frames $\{I_t | t = 1, 2, \dots, B\}$ where $B$ is the batch size that contains $2K+1$ frames and $K$ is the number of pre and post frames from the central frame at $t$. In our experiment, we set $K = 2$, and we used 2 consecutive frame coordinate grids before and after the central frame, making 5 frame coordinate grids plus the central frame. These coordinate grids are passed to the denoiser in a batch of dimension $5 \times \gamma(p_t) \times H \times W$. Each pixel $p_t = (x, y,t)$ in the coordinate grid is passed through a positional encoding $\gamma(.)$ in \eqref{pos}, which maps the low-dimensional coordinates into high-dimension of size $2(x*L)$. We set $L=30$, hence the resulting dimension is 180. We also added the original pixel coordinates to the high-dimension output from the positional encoding. Finally, the input to the feature generator $\mathcal{F}_\theta = 183$.
\begin{equation}
\gamma(\mathbf{p}_t) = [\mathrm{sin}(2^0 \pi \mathbf{p}_t), \mathrm{cos}(2^0 \pi \mathbf{p}_t), ..., \mathrm{sin}(2^{L-1} \pi \mathbf{p}_t), \mathrm{cos}(2^{L-1} \pi \mathbf{p}_t)]
\label{pos}
\end{equation}
The  feature generator $\mathcal{F}_\theta$ has 6 convolution layers with 256 filters in each layer except for the last layer. The output of the last layer is $C$ feature maps where $C = 3 \times B$. The first kernel size of the first convolution layer is kernel size of 1, while the remaining six layers have kernel size of 3. Following the approach of \cite{nerf, mipnerf, rawnerf, fourier}, we chose a kernel size of 1 in the first layer so that we could map the input coordinate to a linear network. For calcium imaging, the output of $\mathcal{F}_\theta$ is $C = 1 \times B$.
\begin{table}[h]
    % \small
    \begin{center}
    \begin{tabular}{ccc}
     \hline
     \centering
      Name &  $N_{out}$  & Function\\ 
      \hline
      Input &  $B*C$  &   \\ 
      conv\_0 &  256  & Convolution 1 x 1 \\
      conv\_1 &  96  & Convolution 1 x 1 \\
      conv\_2 &  $k$  & Convolution 1 x 1 \\
     \hline
    \end{tabular}
    \end{center}
\caption{\textbf{Network architecture of the denoise-net}}
\label{tab:denoise}
\end{table}

The output of the feature generator is passed as input to the denoise-net $\mathcal{D}_\phi$. The batched feature map output from $\mathcal{F}_\theta$ is concatenated to form an input dimension of $1 \times B*C \times H \times W$. The output of the denoise-net is $k$ where $k =3$ for RGB color of the middle frame $t$. For calcium imaging, $k=1$ which is the color channel of the grayscale image. The denoise net has 3 convolution layers with the 256, 96, and $k$ filters for the first, second, and third layers, respectively, as shown in Table \ref{tab:denoise}. All the layers of the model have a kernel size of 1.

\begin{table}[h]
    % \small
    \begin{center}
    \begin{tabular}{ccc}
     \hline
     \centering
      Name &  $H_{out}$  & Function\\ 
      \hline
      Input &  3 &   \\ 
      mlp\_0 &  256  & Linear \\
      mlp\_1 &  256  & Linear \\
      mlp\_2 &  256  & Linear \\
      mlp\_3 &  256  & Linear \\
      mlp\_4 &  $k$  & Linear \\
     \hline
    \end{tabular}
    \end{center}
\caption{\textbf{Network architecture of the refine-net.}}
\label{tab:ablation}
\end{table}
The refine net $\mathcal{F}_\theta$ Sinusoidal Representation Networks (SIREN) \cite{siren} as the backbone. The network takes as input the coordinates of the denoised output from the denoise-net and outputs the refined denoised central frame where each pixel coordinate $p_t = (x,y)$. The network is made up of fully connected layers with 4 linear layers, and the activation at each layer is a sine function. Each linear has 256 hidden units, while the output layer has $k$ nodes, where $k=3$ for RGB and $k=1$ for grayscale.

\vspace{5mm}

\textbf{Training Details:}  Unlike conventional denoising algorithms \cite{udvd, fastdvdnet, self-supervised, dncnn} on synthetic noise, we did not add noise during training. We used fixed noise values throughout the training. We experimented with three different noise types; Gaussian, Poisson, and Impulse types. For Gaussian and Poisson noise types, we used 30 and 50 noise levels and we used noise levels of 0.2 and 0.3 for Impulse noise. To create the noisy version of the clean video sequence, we added noise to frames in the video sequences and saved the noisy frames to a file, this allows us to have a fixed noise value for each frame during training. We simply load these noisy video frames during training instead of adding noise to clean images. We did not use any data augmentation during training.

\vspace{5mm}
\textbf{Optimization Details:} We trained all the sub-networks using Adam \cite{kingma2014adam} optimizer. We trained the Feature generator and Denoise-net jointly by minimizing $l1$ loss between the central channel of the feature map and the corresponding noisy frames for the Feature generator and minimizing the $l1$ loss between the denoised central frame and the corresponding central frame for the denoise-net. $\lambda_1$ in \ref{loss} is set to 1.0, which controls the trade-off between the two loss terms. Where $F_t^{c}$ and $I_t$ are the central channel of the feature map and corresponding noisy frames, while $\hat{I}_B$, and $I^c$ are the denoised central frames and noisy central frame in the input batch respectively 
\begin{equation}
    \mathcal{L}_{1} = ||\hat{I}_B - I^c|| + \lambda_1(\frac{1}{B}\sum_{t=1}^B|| F_t^{c} - I_t)||
    \label{loss}
\end{equation}

We trained a refine-net to further improve the quality of the denoised output from the denoise-net. As shown in \ref{siren_loss}, we minimized $l1$ loss between the output of the refine-net and the output of the denoise-net and $l1$ loss between the refine-net output and the corresponding noisy frame. $\lambda_2$ and $\lambda_3$ are used as regularization terms to balance between details preservation and reducing noise, and the regularization terms were set to 0.1 and 1.0, respectively.

We set the initial learning rate to $0.0001$ set for joint training of the feature generator, and the denoise-net and learning rate of $0.00001$ was used for the refine-net training stage. Both learning rates were reduced by a factor of 10 every 1000 epochs. We froze the weights of the feature generator and denoise-net during the training of the refine-net

\section{Denoising Result}
In this section, we provide additional visual results of our experiments on DAVIS and Set8 datasets corrupted with Gaussian noise with $\sigma = 30$ and $50$, Poisson noise with $\lambda=30$ and $50$ and Impulse with $\alpha = 0.2$. We show our results for bus, hypersmooth, and snowboard.

\section{Ablation Study}
\textbf{Positional encoding.} We provide ablation studies on the input embedding in \ref{posenc} using the bus video sequence in DAVIS dataset. We experimented with different frequency levels to encode the input coordinates. Table \ref{tab:PE} describes the final denoising result of different $L$ on poisson noise level $\lambda = 30$
\begin{table}[h]
    % \small
    \begin{center}
    \begin{tabular}{ccccccc}
     \hline
     \centering
       Metrics &  $L=5$  &  $L=10$ &  $L=20$ &  $L=30$ &  $L=50$ &  $L=100$\\ 
      \hline
      PSNR &   &   &   &   &   &   \\ 
      SSIM &    &  &   &   &   &   \\
     \hline
    \end{tabular}
    \end{center}
\caption{\textbf{Postional encoding ablation} $L$ means frequency level used to encode the low dimensional coordinate to high dimension.}
\label{tab:PE}
\end{table}

We also show the visual output of each stage of our network. Fig \ref{fig:stages} shows the denoising result of the central RGB channel of the feature map output of the feature generator, we also show the result of the denoise-net and finally the refine-net. The result shows that the addition of refine-net significantly improved the denoising result.
